# Supplementary material for: Alternately denoising and reconstructing unoriented point sets
Source: arXiv:2305.00391 source file (2023-08-24)
Supplement: Supplementary file 1 [file supplement_latex.pdf]

# Supplementary material of “Alternately denoising and reconstructing unoriented point sets”

**Table 3. Quantitative comparisons on the famous dataset based on the mean absolute distance-to-surface (MADS) of each method. The MADS values are multiplied by  $10^3$ .**

| Method/STD      | $0.5 \times 10^{-2}$ | $1.0 \times 10^{-2}$ | $1.5 \times 10^{-2}$ | $2.0 \times 10^{-2}$ | $2.5 \times 10^{-2}$ |
|-----------------|----------------------|----------------------|----------------------|----------------------|----------------------|
| RIMLS           | 2.015                | 2.480                | 3.350                | 4.804                | 7.129                |
| WLOP            | 2.684                | 2.874                | 3.126                | 3.508                | 4.162                |
| Bilateral-small | 1.721                | 2.214                | 2.974                | 4.059                | 5.517                |
| Bilateral-large | 2.954                | 3.269                | 3.634                | 3.999                | 4.590                |
| Jet-small       | <b>1.592</b>         | 2.159                | 2.855                | 3.799                | 5.011                |
| Jet-large       | 2.126                | 2.599                | 3.081                | 3.636                | 4.365                |
| PointCleanNet   | 1.979                | 2.592                | 3.108                | 3.633                | 4.196                |
| Ours            | 1.624                | <b>1.840</b>         | <b>2.074</b>         | <b>2.655</b>         | <b>3.275</b>         |

**Table 4. Quantitative comparisons of the reconstructed mesh quality based on the F-score with the threshold  $5 \times 10^{-3}$ . The red color is used to represent the best value amongst all approaches, and the blue is used to denote the second best.**

| Model         | Noise                | RIMLS        | WLOP  | Bilateral-small | Bilateral-large | Jet-small    | Jet-large    | PointCleanNet | Ours         |
|---------------|----------------------|--------------|-------|-----------------|-----------------|--------------|--------------|---------------|--------------|
| tortuga       | $0.5 \times 10^{-2}$ | 0.996        | 0.971 | <b>0.997</b>    | 0.919           | <b>0.999</b> | <b>0.999</b> | <b>0.999</b>  | <b>0.999</b> |
| Utah_teapot   | $0.5 \times 10^{-2}$ | <b>0.991</b> | 0.931 | <b>0.995</b>    | 0.961           | 0.987        | 0.979        | 0.981         | 0.989        |
| horse         | $1.0 \times 10^{-2}$ | 0.964        | 0.846 | <b>0.999</b>    | 0.939           | 0.997        | 0.993        | 0.993         | <b>0.998</b> |
| angle         | $1.0 \times 10^{-2}$ | 0.921        | 0.757 | <b>0.990</b>    | 0.866           | <b>0.983</b> | 0.954        | 0.951         | <b>0.990</b> |
| Armadillo     | $1.5 \times 10^{-2}$ | 0.732        | 0.855 | 0.886           | 0.616           | <b>0.909</b> | 0.859        | 0.908         | <b>0.949</b> |
| xyzrgb_dragon | $1.5 \times 10^{-2}$ | 0.550        | 0.678 | <b>0.883</b>    | 0.660           | 0.875        | 0.775        | 0.833         | <b>0.914</b> |
| hand          | $2.0 \times 10^{-2}$ | 0.206        | 0.413 | 0.761           | 0.522           | <b>0.835</b> | 0.678        | 0.727         | <b>0.803</b> |
| serapis       | $2.0 \times 10^{-2}$ | 0.759        | 0.841 | <b>0.901</b>    | 0.828           | 0.887        | 0.861        | 0.879         | <b>0.916</b> |
| Liberty       | $2.5 \times 10^{-2}$ | 0.120        | 0.652 | 0.606           | 0.769           | 0.681        | 0.817        | <b>0.854</b>  | <b>0.840</b> |
| galera        | $2.5 \times 10^{-2}$ | 0.428        | 0.793 | 0.813           | 0.698           | <b>0.833</b> | 0.797        | 0.825         | <b>0.869</b> |

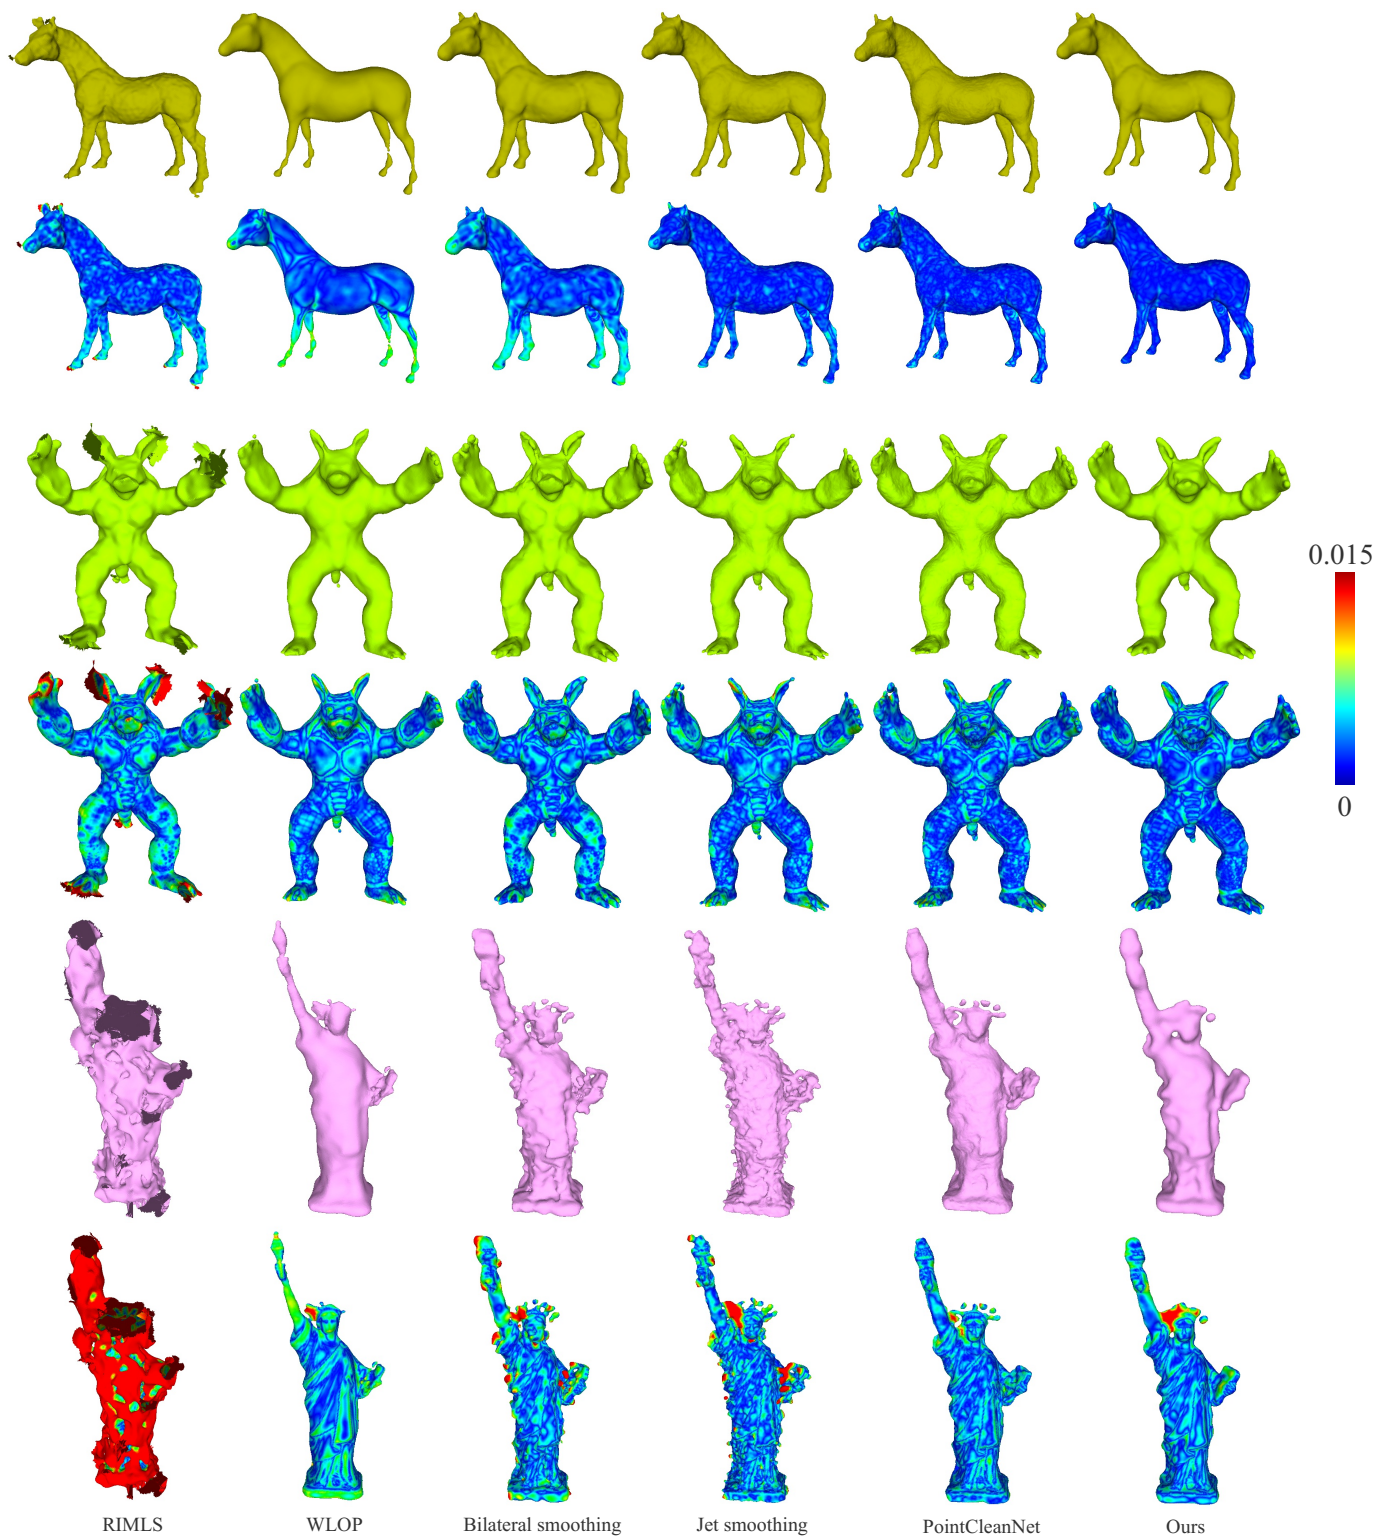

Fig. 15. Qualitative comparisons of the reconstructed mesh amongst different methods. The results indicate that our approach exhibits well-rounded performance.
